# Supplementary material for: Clinical Note Bloat Reduction for Efficient LLM Use
Source: arXiv:2604.16364 source file (2026-10-26)
Supplement: Supplementary file 1 [file SI-main.tex]

\documentclass[letterpaper]{SI/nature}

%% CUSTOM DEFINITIONS  
\usepackage{color}
\usepackage{colortbl}
\usepackage{url}
\usepackage{verbatim}
\usepackage{multirow}
\usepackage{xspace}
\usepackage{graphicx}
\usepackage{amsmath} 
\usepackage{amssymb}
\usepackage{booktabs} 
\usepackage{times} 
\usepackage{enumitem}
\usepackage{xcolor}
\usepackage{placeins} 
\usepackage{rotating}
\usepackage{chngcntr}
\usepackage{lineno}
\usepackage{tcolorbox}
\usepackage{csvsimple}

\usepackage[colorlinks,citecolor=blue,urlcolor=magenta]{hyperref}
\urlstyle{same}

\usepackage[labelfont=bf, font=footnotesize]{caption}
\usepackage[left=0.9in,right=0.9in]{geometry}
\usepackage{longtable}
\usepackage{lscape}
\usepackage{subcaption}
\usepackage{array}
\usepackage{mwe}
\usepackage{comment}

\usepackage{siunitx}

\let\oldnl\nl
\newcommand{\nonl}{\renewcommand{\nl}{\let\nl\oldnl}}

\makeatletter
\makeatother

\makeatletter
\makeatother
\newcolumntype{L}[1]{>{\raggedright\let\newline\\\arraybackslash\hspace{0pt}}m{#1}}

\setlength{\tabcolsep}{3pt}
\definecolor{Gray}{gray}{0.85}
\newcolumntype{b}{>{\columncolor{blue!20}}l}  % c --> l
\newcolumntype{a}{>{\columncolor{Gray}}l}  % c --> l

% To hide column
\usepackage{array}
\newcolumntype{H}{>{\setbox0=\hbox\bgroup}c<{\egroup}@{}}

\graphicspath{{./FIG/}}

\title{}
\author{}
 
\begin{document}

\maketitle
\thispagestyle{empty}
\spacing{1.3}

\begin{center}
{\Large Supplementary Information for\\[3mm]
{\bf Clinical Note Bloat Reduction for Efficient LLM Use}\\[3mm]}
\end{center}

\author  
{\begin{center}   
Jordan L. Cahoon$^{1,2,*}$, Chloe O. Stanwyck$^{1,3,*}$\textbf{}, Asad Aali$^{4}$, Rachel Madding$^{5}$, Emma Sun$^{1}$, Yixing Jiang$^{1}$, Renumathy Dhanasekaran$^{6}$, and Emily Alsentzer$^{1,7,8,\ddag}$ \\[1mm]  
\small{$^{1}$Department of Biomedical Data Science, Stanford University, Stanford, CA} \\
\small{$^{2}$Department of Pathology, Stanford University, Stanford,
CA} \\
\small{$^{3}$Department of Anesthesiology, Perioperative and Pain Medicine, Stanford University, Stanford,
CA} \\
\small{$^{4}$Department of Radiology, Stanford University, Stanford,
CA} \\
\small{$^{5}$Department of Obstetrics and Gynecology, Stanford University, Stanford,
CA} \\
\small{$^{6}$Division of Gastroenterology and
Hepatology, Stanford University, Stanford,
CA} \\
\small{$^{7}$Department of Computer Science, Stanford University, Stanford, CA} \\
\small{$^{8}$Weill Cancer Hub West} \\
[1mm]
\small{$\ddag$Corresponding author. Email: ealsentzer@stanford.edu}\\
\small{$^*$Equal contribution} 
\end{center}
}

{\spacing{1}

\clearpage

\section*{Supplementary Notes}
\input{SI/SI-notes}

\newpage
\section*{Supplementary Figures and Tables}
\input{SI/SI-figures}
\end{document}
